# Supplementary material for: Transport of spatial quantum correlations through an optical waveguide
Source: arXiv:1712.07451 ancillary file (2017-12-20)
Supplement: Supplementary file 1 [file suppl_info_v3.pdf]

# Transport of spatial quantum correlations through an optical waveguide: supplementary information

J. Hordell, D. Benedicto-Orenes, P. G. Petrov, A. U. Kowalczyk, G. Barontini, and V. Boyer
*Midland Ultracold Atom Research Centre, School of Physics and Astronomy,*
*University of Birmingham, Edgbaston, Birmingham B15 2TT, UK*

## I. LOSSES

The conduit has a transmission of around 30%. This leads to an imbalance between the probe and conjugate signals and a sub-optimal subtraction of the common amplification noise. For practical reasons, we use a perfectly balanced photodetector, which subtracts the photocurrent before trans-amplification. This prevents us from applying a different trans-amplification gain on both signals in order to re-balance them. We therefore impose a certain amount of attenuation on the conjugate beam path, with a tunable beamsplitter optimised to conserve the maximum amount of intensity-difference squeezing.

Losses on both beam paths, including finite transmission by the conduit, losses on lenses and mirrors, balancing beamsplitter on the conjugate and finite quantum efficiency of the detector, are modelled by a single beamsplitter on each beam, whose effect is to attenuate the beam and inject vacuum noise [1]. The four-wave mixing amplification and loss model is presented in Fig.**??**(a). The field operators at detection are:

$$\begin{aligned} \hat{a}'' &= \sqrt{GT_a}\ \hat{a} - \sqrt{(G-1)T_a}\ \hat{b}^\dagger + \sqrt{1-T_a}\ \hat{c} \\ \hat{b}'' &= -\sqrt{(G-1)T_b}\ \hat{a}^\dagger + \sqrt{GT_b}\ \hat{b} + \sqrt{1-T_b}\ \hat{d}, \end{aligned} \tag{1}$$

where $\hat{a}$ is the annihilation operator of the input probe field, $\hat{b}$ is the same for input conjugate field, $\hat{c}$ and $\hat{d}$ are the loss annihilation operators coupled to the probe and conjugate fields via beamsplitters with transmission $T_a$ and $T_b$, and $G$ is the four-wave-mixing gain. This leads to the variance in the differential number of detected photons $\hat{n}_- = \hat{n}_a'' - \hat{n}_b''$ for a coherent state $|\alpha\rangle$ on input $a$ and a vacuum $|0\rangle$ on input $b$:

$$\langle(\Delta\hat{n}_-)^2\rangle = \{[GT_a - T_b(G-1)]^2 + G(G-1)(T_b-T_a)^2 + GT_a(1-T_a) + (G-1)T_b(1-T_b)\}|\alpha|^2. \tag{2}$$

The shot noise is given by the mean number of photons of the probe and conjugate at the detector $\langle\hat{n}_+\rangle = \hat{n}_a'' + \hat{n}_b''$ and can be written as

$$\langle\hat{n}_+\rangle = [GT_a + (G-1)T_b]|\alpha|^2. \tag{3}$$

Finally for the squeezing parameter in dB units we get:

$$S = 10\log_{10}\left[\frac{\langle(\Delta\hat{n}_-)^2\rangle}{\langle\hat{n}_+\rangle}\right]. \tag{4}$$

It is possible to maximise the amount of detected squeezing, that is to say the to minimise the amount of intensity difference noise relative to shot noise [Eq.(4)] in both the gain $G$ and the conjugate transmission $T_b$. For a overall probe transmission $T_a = 0.3$, the optimum values are found to be $G = 1.3$ and $T_b = 1$, resulting in a theoretical 1.65 dB of squeezing. The squeezing varies very softly with these parameters and in practice we choose a gain $G \approx 1.5$ at the centre of the pump beam and a transmission $T_b = 0.75$ for a theoretical squeezing of 1.63 dB below shot noise [see Fig.**??**(b)].

A value close to this amount of squeezing is observed when measuring the squeezing on the intensity difference of the whole beams (about -1.5dB). The measured degree of squeezing when using the slits is lower than this value however. This is due to the fact that the transmission function of the slits lays partially outside the spatial bandwidth of the 4WM process, both because the slits width is of the order of the coherence length, and because their transmission functions contains high spatial frequencies due to their sharp edges. Furthermore, optical aberrations may contribute to reduced measured correlations.

---

[1] C. Caves and D. Crouch, "Quantum wideband traveling-wave analysis of a degenerate parametric amplifier," J. Opt. Soc. Am. B 4, 1535-1545 (1987).

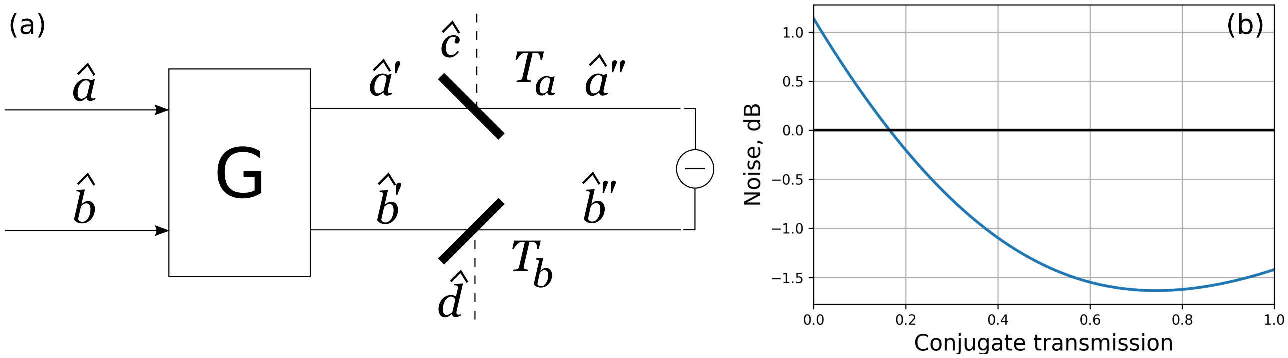


FIG. 1. Theoretical model of losses in the experiment. (a) The FWM medium has a gain of $G$. The input probe and conjugate annihilation operators are depicted by $\hat{a}$ and $\hat{b}$. After the amplification the operators are $\hat{a}^{'}$ and $\hat{b}^{'}$ and after mixing vacuum fields $\hat{c}$ and $\hat{d}$ at beamsplitters with transmission $T_a$ and $T_b$ the operators are transformed to $\hat{a}^{''}$ and $\hat{b}^{''}$. (b) Optimization of conjugate transmission. The probe transmission is 0.3 and the maximum squeezing for a gain of 1.5 can be seen to happen at transmission of the conjugate of 0.75. The solid black line is the shot noise.
